# Supplementary material for: Identification of multi-valued treatment effects with unobserved heterogeneity
Source: arXiv:2010.04385 source file (2023-04-26)
Supplement: Supplementary file 3 [file settings_supp.tex]

\usepackage[utf8]{inputenc}

\usepackage{amsthm,amsmath,amssymb}
\if0
\usepackage{mathtools}
\mathtoolsset{showonlyrefs}
\fi
\usepackage{letterspace}
\usepackage{graphicx}
\usepackage{setspace}
\usepackage{ascmac}
\usepackage{bm}

\usepackage{xcolor}

\usepackage{filecontents}
\makeatletter\@input{ivqr_id_a.tex}\makeatother

\usepackage{nameref} % これが\zexternaldocumentの前までに必要
\usepackage{zref-xr}
\zxrsetup{toltxlabel} % 通常のLaTeXスタイルの\refを使う（\zexternaldocumentより前におく）
%\zexternaldocument*[1:]{ivqr_id} % \zのついたexternaldocumentを使う
\zexternaldocument*{ivqr_id}

\if0
\usepackage{xr}
\externaldocument{ivqr_id}% article1内の\labelを取り込む

\usepackage{xr}
\makeatletter
\newcommand*{\addFileDependency}[1]{% argument=file name and extension
  \typeout{(#1)}
  \@addtofilelist{#1}
  \IfFileExists{#1}{}{\typeout{No file #1.}}
}
\makeatother

\newcommand*{\myexternaldocument}[1]{%
    \externaldocument{#1}%
    \addFileDependency{#1.tex}%
    \addFileDependency{#1.aux}%
}
\myexternaldocument{ivqr_id}
\fi

\usepackage{algorithm2e}
\usepackage{algorithmic}
\usepackage{enumitem}
\usepackage{latexsym}

\if0

\fi

\if0
\setlength{\footnotesep}{18pt}
\makeatletter
\let\@makefntextOrig\@makefntext
\def\@makefntext#1{\@makefntextOrig{%
\baselineskip=18pt%%%ここで脚注の行間隔を指定
#1}}
\makeatother
\fi

%\linespread{1.3}

\theoremstyle{plain}% default

\theoremstyle{definition}

\usepackage[top=1.25in, bottom=1.25in, left=1.25in, right=1.25in]{geometry}

\onehalfspacing

\numberwithin{equation}{section}

\usepackage{color}

% 数式(演算子など)のスペースを詰める
% =,→ 間の余白
\thickmuskip=1.0\thickmuskip
% +,- 間の余白
\medmuskip=0.8\medmuskip
% … などの装飾記号の余白
\thinmuskip=0.8\thinmuskip
% 行列を詰める
\arraycolsep=0.3\arraycolsep
% 数式の上下のスペースの変更
\AtBeginDocument{
  \abovedisplayskip     =0.6\abovedisplayskip
  \abovedisplayshortskip=0.6\abovedisplayshortskip
  \belowdisplayskip     =0.6\belowdisplayskip
  \belowdisplayshortskip=0.6\belowdisplayshortskip}

\let\oldenumerate\enumerate
\renewcommand{\enumerate}{
\oldenumerate
\setlength{\itemsep}{1.5pt}
\setlength{\parskip}{1.5pt}
\setlength{\parsep}{1.5pt}
}

\sloppy

\setcounter{section}{3}

\setcounter{lemma}{7}

\setcounter{remark}{2}

\usepackage{hyperref}
\hypersetup{
       colorlinks=false,
       citebordercolor=green,
       linkbordercolor=red,
       urlbordercolor=cyan,
}
\usepackage{breakcites}
\usepackage{breakurl}
\usepackage[authoryear, round]{natbib}
\bibliographystyle{econometrica}
